# Supplementary material for: Strong enhancement of magnetic order from bulk to stretched monolayer FeSe as Hund's metals
Source: arXiv:2009.02024 source file (2020-09-04)
Supplement: Supplementary file 1 [file SI.pdf]

# Supplementary Information

## Strong enhancement of magnetic order from bulk to stretched monolayer FeSe as Hund's metals

Chang-Youn Moon

*Quantum Technology Institute, Korea Research Institute of Standards and Science, Yuseong, Daejeon 305-340, Republic of Korea*

## Supplementary Note 1: Orbital susceptibility

The orbital susceptibility is defined as $\chi_{orb} = \chi^c_{xz;xz} + \chi^c_{yz;yz} - 2\chi^c_{xz;yz} \propto \langle (n_{xz} - n_{yz})(n_{xz} - n_{yz}) \rangle$, where $\chi^c_{\alpha;\beta}$ is the charge susceptibility in the $\alpha - \beta$ orbital channel. The imaginary part of $\chi_{orb}$ is displayed for the three materials in Supplementary Figure 1. Low energy fluctuations are very weak compared with high energy ones regardless of materials, with only traces of low energy modes near $q = (0, 0)$ and $(1, 0)$, which might be associated with the 'ferro orbital order'[1–3] and other spatially non-uniform orbital orders suggested theoretically[4–7]. As pointed out by Fanfarillo *et al.*[7], orbital orders are not stabilized by the inclusion of local correlations in these materials in which Hund's coupling prefers the degeneracy between $d_{xz}$ and $d_{yz}$ orbitals, whereas an orbital order is generally set by the tendency of charge localization to avoid Coulomb repulsion. While the inclusion of non-local correlation effects might help stabilize an orbital order in some of iron-based superconductors, DFT+DMFT scheme is found not to support the existence of orbital orders in these materials.

## Supplementary Note 2: Possible effects of using material-specific $U$ and $J$

In the DFT+DMFT scheme adopted in this work, $U$ and $J$ are larger and more similar among various IBS due to weaker screening of the Coulomb interaction by using more localized quasi-atomic orbitals as correlated basis set, compared with more traditional schemes using Wannier basis set. Therefore, we use the same $U = 5.0$ eV and $J = 0.8$ eV values for all of the three materials, which were determined for $BaFe_2As_2$ by a self-consistent GW calculation[8]. Nevertheless, if $U$ and $J$ are explicitly evaluated for each material, larger values are likely for bulk and ML FeSe than LaFeAsO, although the variation of values are expected to be minimal over the three materials (see Ref. 23 in the main text). Using material-specific $U$ and $J$, then, the suppression of magnetic order in bulk FeSe compared with LaFeAsO could possibly become less obvious. However, even in that case, one of our main conclusions, that the enhanced orbital decoupling in bulk FeSe by a large crystal field splitting between $e_g$ and $t_{2g}$ orbitals contributes to suppress magnetic ordering, does not change. As for the monolayer FeSe, a stronger magnetic order might be realized and our conclusion of the proximity of the magnetic order to the superconductivity and discussion

on the compatible superconducting mechanism in monolayer FeSe on STO substrate would not change.

## Supplementary Note 3: Orbital-resolved spin fluctuation

Orbital-resolved spin fluctuation $\langle S^z_\alpha S^z_\beta \rangle - \langle S^z_\alpha \rangle \langle S^z_\beta \rangle$ where $\alpha$ and $\beta$ are orbital indexes, is estimated and listed in Supplementary Table 1. Regardless of the orbital decoupling in charge degree of freedom, Hund's coupling enforces the parallel spin alignment among orbitals in IBS, meaning that orbitals are always strongly coupled in the spin degree of freedom. As a result, Supplementary Table 1 shows that inter-orbital spin fluctuations do not change as much as the charge counterparts over materials in Table 1 in the main text, and one can see that the variation of inter-orbital spin fluctuation over materials between two specific orbitals mostly follow that of the two respective intra-orbital components which are again determined by respective orbital occupations shown in Fig. 2c in the main text.

## Supplementary Note 4: Strong $J$-dependence of orbital selectivity

In our conclusion that stronger suppression of the inter-orbital charge fluctuation in bulk FeSe originates from the larger crystal field splitting than LaFeAsO, one should be cautious not to mistake it for that the crystal field splitting itself is the driving force of the Hund's phenomenology. In fact, it is the Hund's coupling that makes the larger orbital crystal field splitting manifested as enhanced orbital decoupling and orbital selectivity, which is represented by the contrast of mass enhancement among orbitals. To demonstrate the strong effect of Hund's coupling in the orbital selectivity, we compare the degree of enhancement of the orbital selectivity between bulk FeSe and LaFeAsO using different values of Hund's coupling $J$. In Supplementary Figure 2a, mass enhancement is displayed for LaFeAsO and bulk FeSe using $U$=5.0 eV and $J$=0.8 eV, as also shown in Fig. 2a in the main text. For a given difference of the orbital crystal field splitting between 0.25 eV and 0.48 eV for LaFeAsO and bulk FeSe, respectively, and also corresponding difference in the orbital occupations as shown in Fig. 2c in the main text, orbital selectivity in bulk FeSe is clearly enhanced compared with that in LaFeAsO. The mass enhancement values of orbitals in bulk FeSe are scattered within a range of about 0.8 (from 2.0 to 2.8), which is over four times larger than the corresponding range in LaFeAsO which is less than 0.2. In contrast, when $J$

is reduced by half to be 0.4 eV in Supplementary Figure 2b, it is clear that the difference of orbital selectivity between two materials are much reduced, apart from the overall decrease of mass enhancement of each orbital from $J$=0.8 eV case shown in Supplementary Figure 2a. For comparison, we also consider the effect of $U$ reduction in Supplementary Figure 2c. In spite of much larger reduction of absolute value of $U$ (by 2.5 eV) than the case of $J$ reduction (by 0.4 eV) in Supplementary Figure 2b from the reference case in Supplementary Figure 2a, the overall mass enhancements are larger and the orbital selectivity difference between the two materials is also much more discernible for $U$=2.5 eV case than $J$=0.4 eV case. This result confirms the vital role of Hund's coupling in the orbital selectivity physics as well as in the overall correlation strength in Hund's metals, as expected.

---

[1] Kruger, F., Kumar, S., Zaanet, J. & van den Brink, J. Spin-orbital frustrations and anomalous metallic state in iron-pnictide superconductors. *Phys. Rev. B* **79**, 054504 (2009).

[2] Lv, W., Wu, J. & Phillips, P. Orbital ordering induces structural phase transition and the resistivity anomaly in iron pnictides. *Phys. Rev. B* **80**, 224506 (2009).

[3] Lee, C.-C., Yin, W.-G. & Ku, W. Ferro-Orbital Order and Strong Magnetic Anisotropy in the Parent Compounds of Iron-Pnictide Superconductors. *Phys. Rev. Lett.* **103**, 267001 (2009).

[4] Chubukov, A. V., Khodas, M. & Fernandes, R. M. Magnetism, Superconductivity, and Spontaneous Orbital Order in Iron-Based Superconductors: Which Comes First and Why? *Phys. Rev. X* **6**, 041045 (2016).

[5] Su, Y., Liao, H. & Li, T. The form and origin of orbital ordering in the electronic nematic phase of iron-based superconductors. *J. Phys. Condens. Matter* **27**, 105702 (2015).

[6] Jiang, K., Hu, J., Ding, H. & Wang, Z. Interatomic Coulomb interaction and electron nematic bond order in FeSe. *Phys. Rev. B* **93**, 115138 (2016).

[7] Fanfarillo, L., Giovannetti, G., Capone, M. & Bascones, E. Nematicity at the Hund's metal crossover in iron superconductors. *Phys. Rev. B* **95**, 144511 (2017).

[8] Kutepov, A., Haule, K., Savrasov, S. Y. & Kotliar, G. Self-consistent *GW* determination of the interaction strength: Application to the iron arsenide superconductors. *Phys. Rev. B* **82**, 045105 (2010).

**Supplementary Table 1:** Orbital-resolved spin fluctuations in the PM phase. A number in a parenthesis represents the inter-orbital element between $d_{xz}$ and $d_{yz}$ orbitals, and the number in front of it is the intra-orbital element of $d_{xz}$ and $d_{yz}$, which are the same.

| | $z^2$ | $x^2-y^2$ | $xz/yz$ | $xy$ |
|---|---|---|---|---|
| | LaFeAsO | | | |
| $z^2$ | 0.276 | 0.139 | 0.136 | 0.139 |
| $x^2-y^2$ | 0.139 | 0.303 | 0.144 | 0.160 |
| $xz/yz$ | 0.136 | 0.144 | 0.307(0.163) | 0.144 |
| $xy$ | 0.139 | 0.160 | 0.144 | 0.301 |
| | bulk FeSe | | | |
| $z^2$ | 0.251 | 0.113 | 0.129 | 0.137 |
| $x^2-y^2$ | 0.113 | 0.277 | 0.138 | 0.159 |
| $xz/yz$ | 0.129 | 0.138 | 0.322(0.178) | 0.167 |
| $xy$ | 0.137 | 0.159 | 0.167 | 0.329 |
| | Monolayer FeSe | | | |
| $z^2$ | 0.270 | 0.130 | 0.141 | 0.153 |
| $x^2-y^2$ | 0.130 | 0.289 | 0.149 | 0.170 |
| $xz/yz$ | 0.141 | 0.149 | 0.323(0.184) | 0.176 |
| $xy$ | 0.153 | 0.170 | 0.176 | 0.334 |

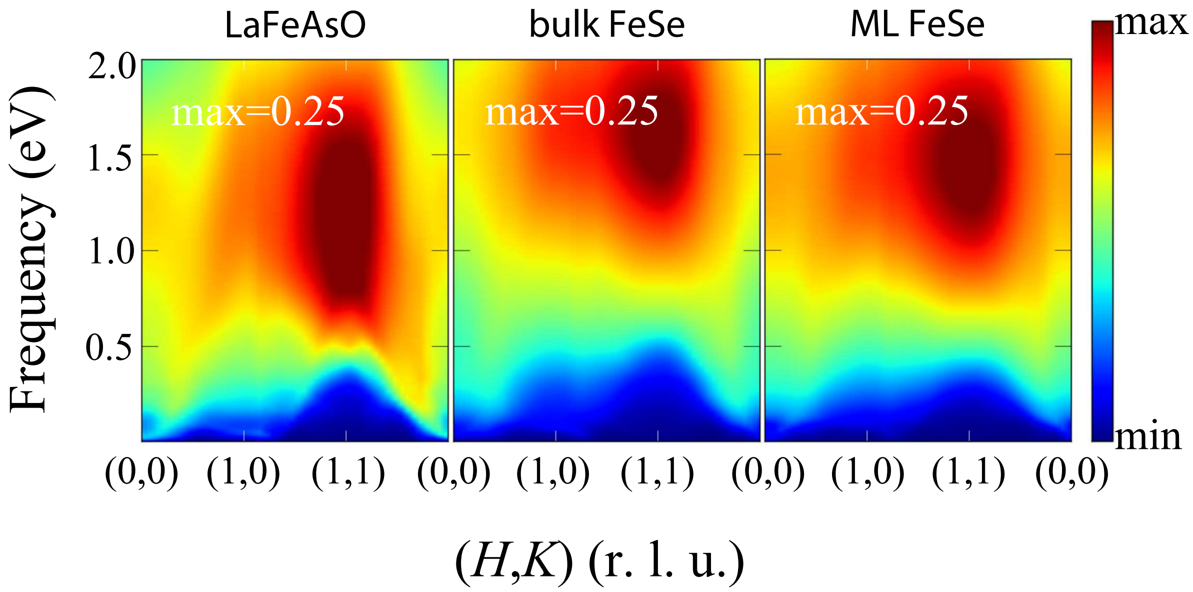


**Supplementary Figure 1:** Imaginary part of the orbital susceptibilities, $\chi''_{orb}$ for LaFeAsO, bulk FeSe, and ML FeSe. $x$-axis is for the momentum transfer $\mathbf{q} = (H, K, L = 1)$ in the reciprocal lattice unit (r. l. u.) of one-Fe-unitcell, and $y$-axis is for the frequency.

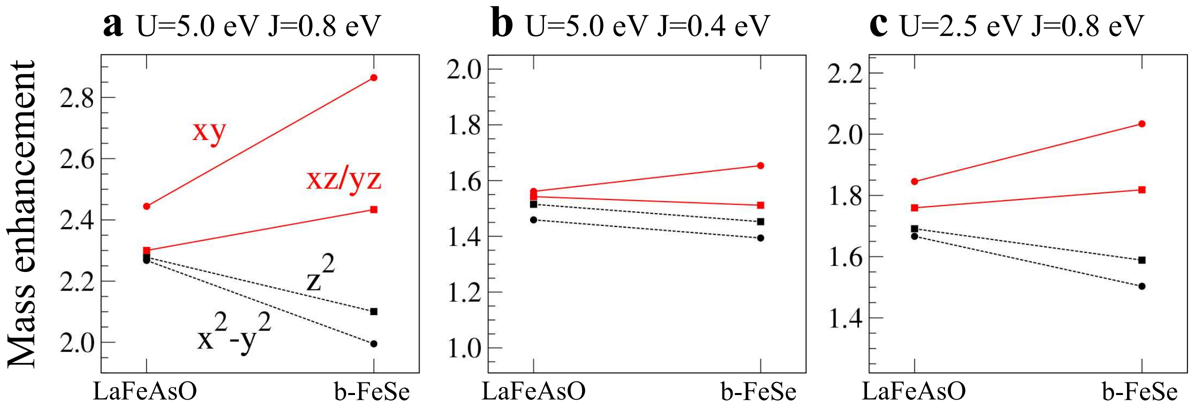


**Supplementary Figure 2:** Orbital-resolved mass enhancement of LaFeAsO and bulk FeSe (b-FeSe) using **a**, $U = 5.0$ eV and $J = 0.8$ eV same as in the main text, **b**, $U = 5.0$ eV and $J = 0.4$ eV, and **c**, $U = 2.5$ eV and $J = 0.8$ eV. Same scale is used for $y$-axes of all the plots to facilitate the comparison.
